# Supplementary material for: Automatic topography of high-dimensional data sets by non-parametric Density Peak clustering
Source: arXiv:1802.10549 ancillary file (2021-02-05)
Supplement: Supplementary file 1 [file SI.pdf]

# Supplementary Information for: Automatic topography of high-dimensional data sets by non-parametric Density Peak clustering

Maria d'Errico,[1] Elena Facco,[1] Alessandro Laio,[1,2,*] and Alex Rodriguez[1,†]

[1] *SISSA,Scuola Internazionale Superiore Studi Avanzati, via Bonomea 265, I-34136 Trieste, Italy*

[2] *ICTP, International Centre for Theoretical Physics, Strada Costiera 11, I-34100, Trieste, Italy*

(Dated: February 28, 2018)

* laio@sissa.it

† alexrod@sissa.it

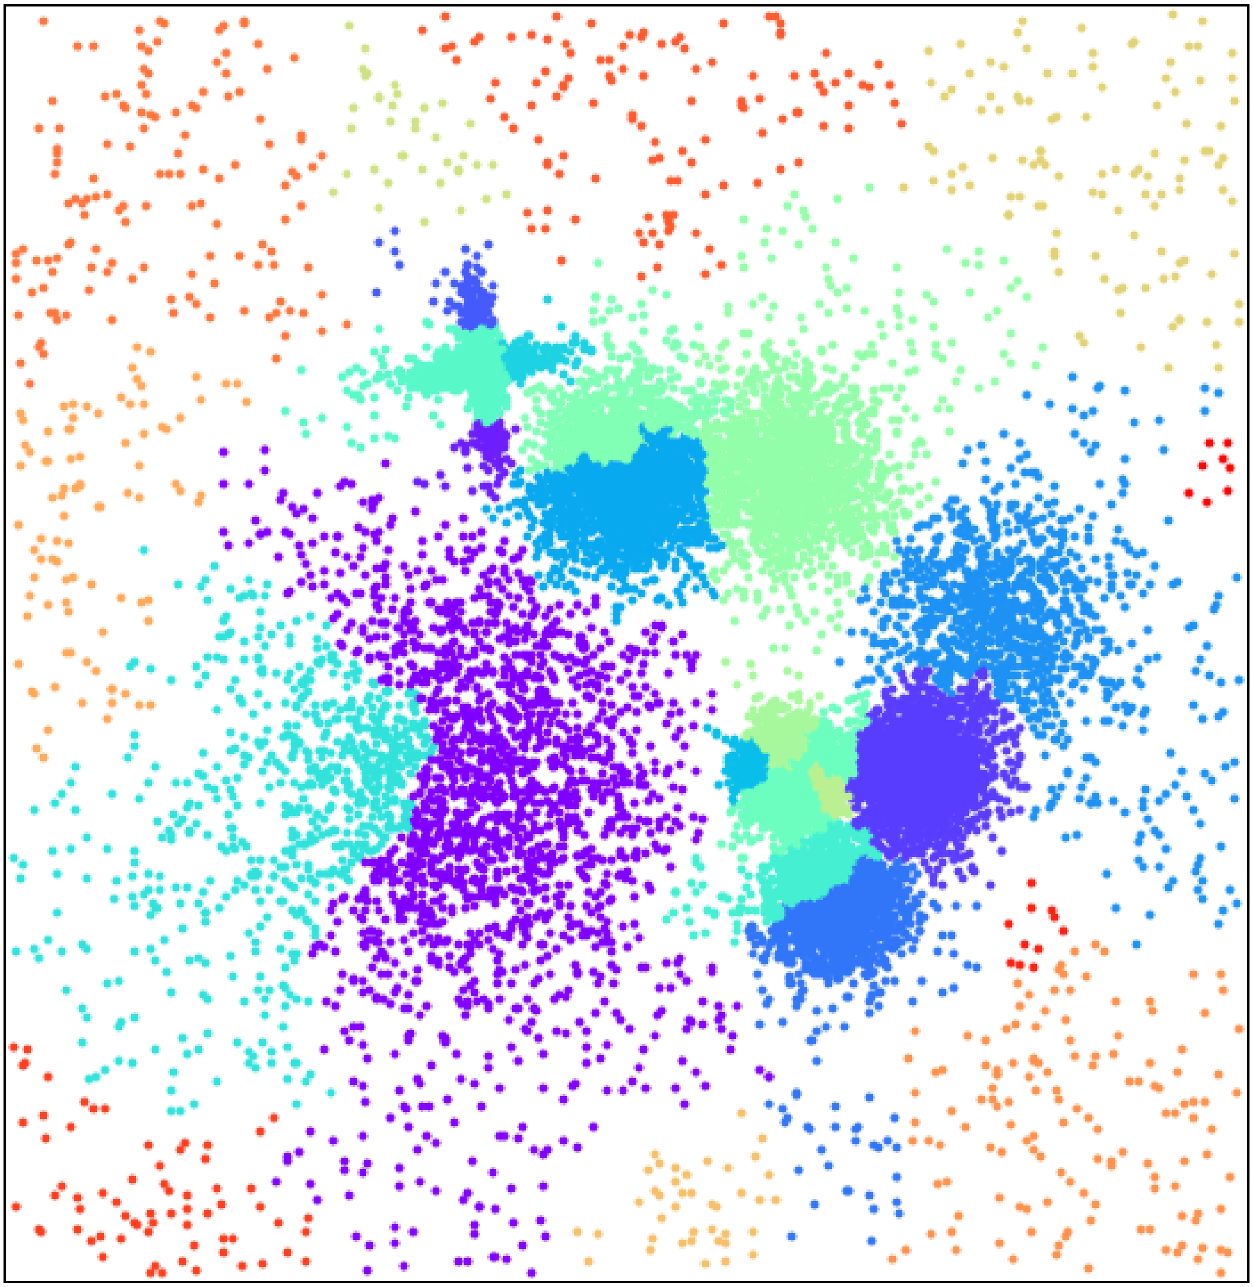

FIG. S1. Automatic assignation of the data set shown in FIG. 1. before spurious clusters are merged. Different colors represent different clusters.

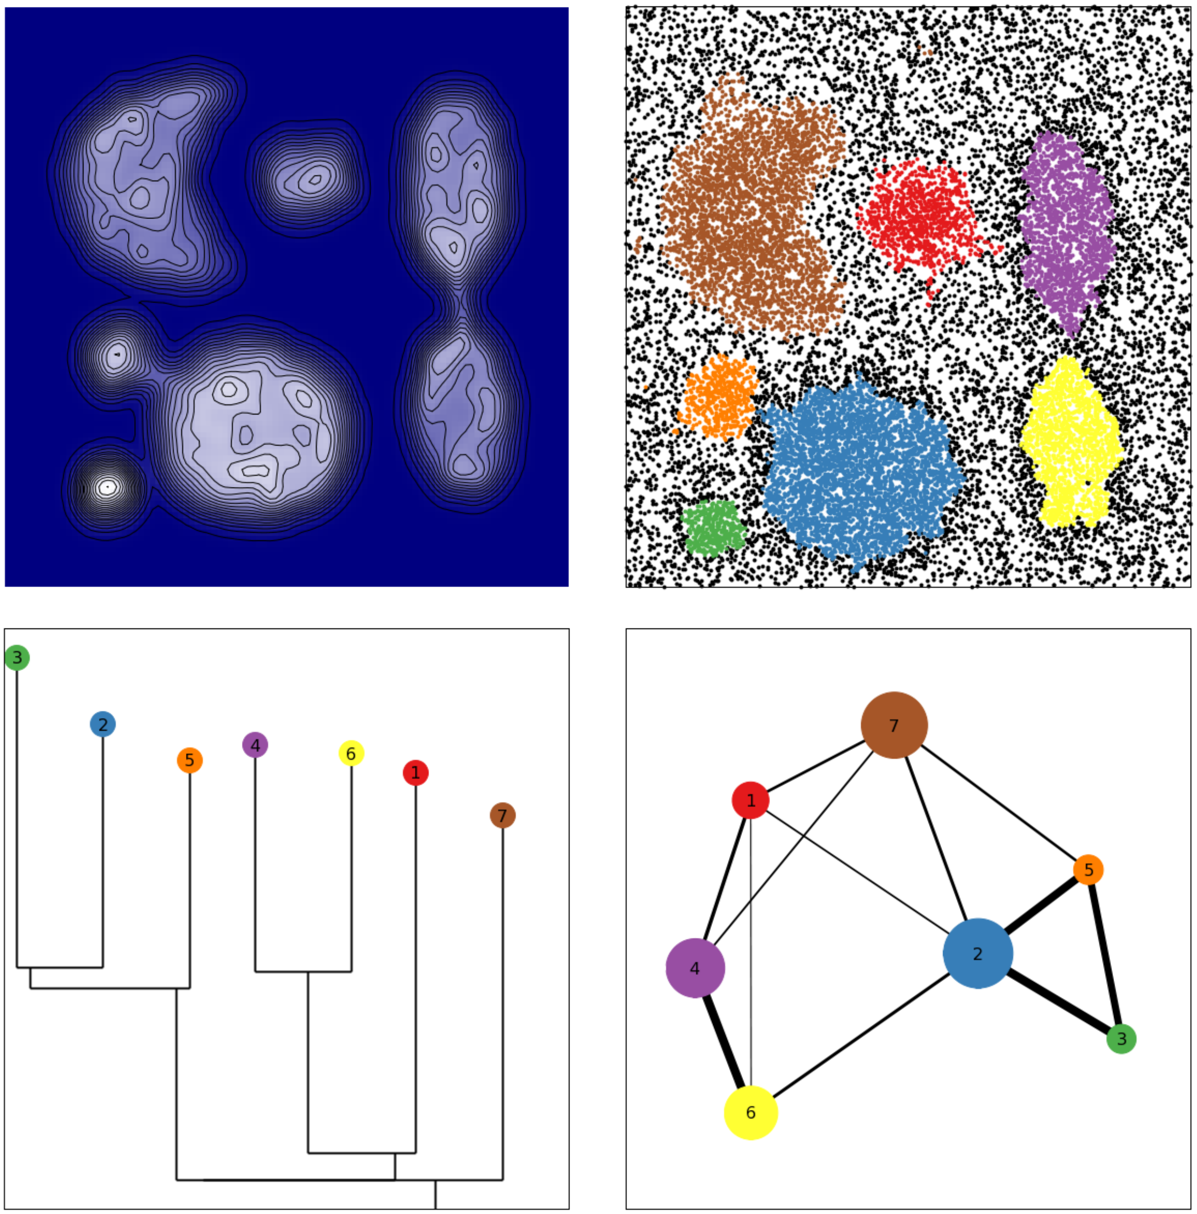


FIG. S2. Analysis of the topography of the Aggregation [1] data set. A total of 20000 points has been harvested from the probability distribution function shown in the top-left panel, built as a sum of Gaussian functions centered in the original data points. The clusters found with a value of $Z = 2.5$ are shown in top-right panel. The dendrogram and network representations of the topography are in the bottom-left and bottom-right panels respectively.

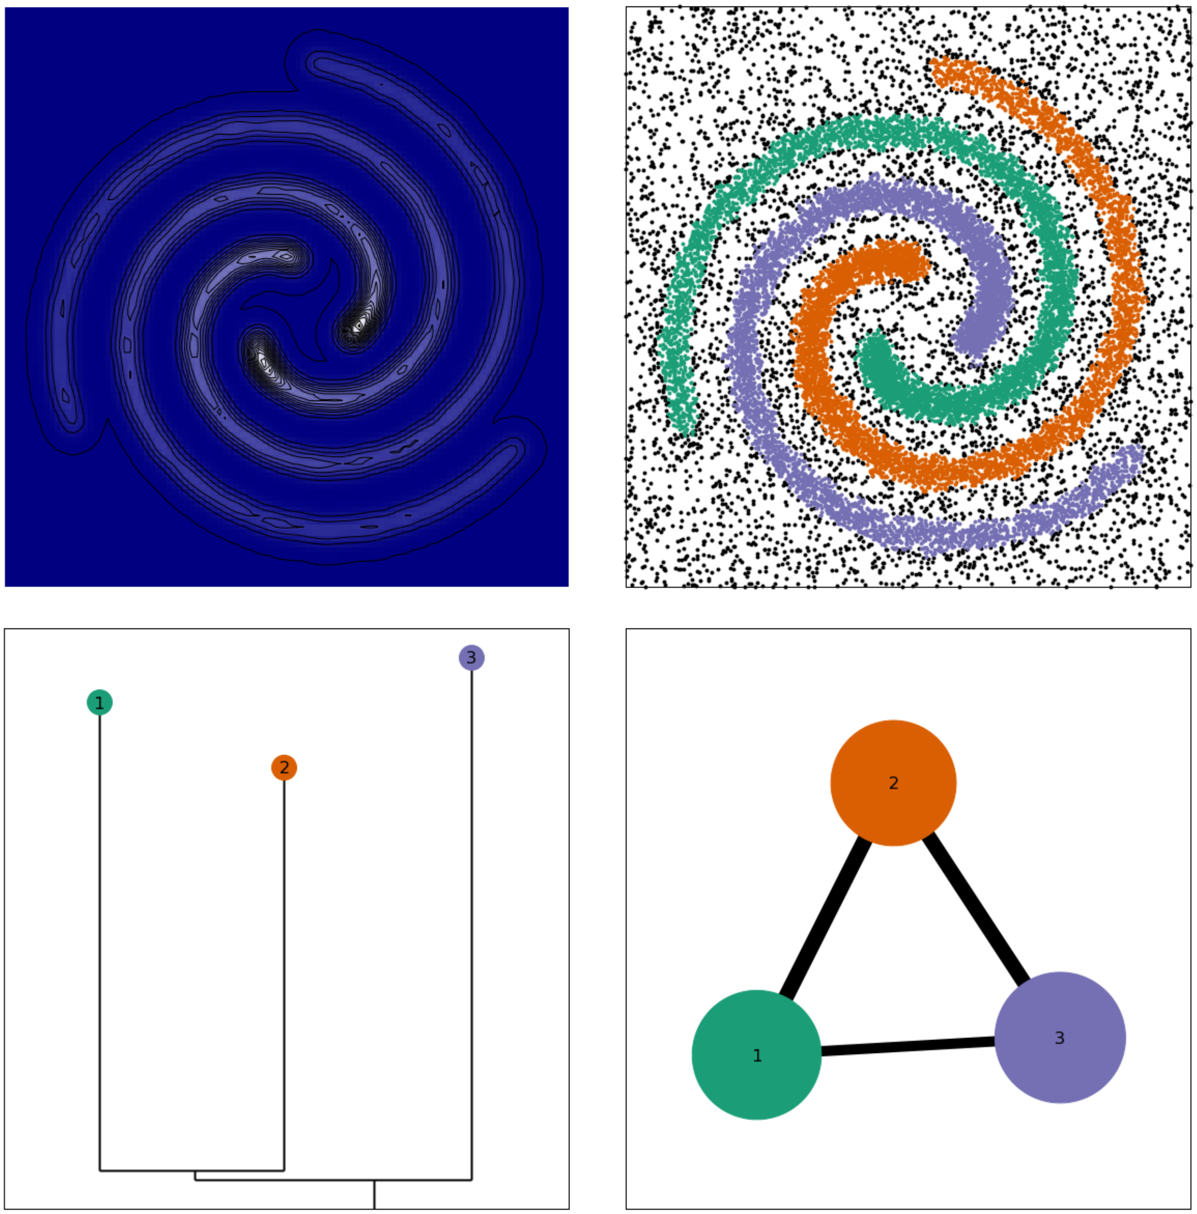


FIG. S3. Analysis of the topography of the Spiral [2] data set. A total of 20000 points has been harvested from the probability distribution function shown in the top-left panel, built as a sum of Gaussian functions centered in the original data points. The clusters found with a value of $Z = 2.7$ are shown in top-right panel. The dendrogram and network representations of the topography are in the bottom-left and bottom-right panels respectively.

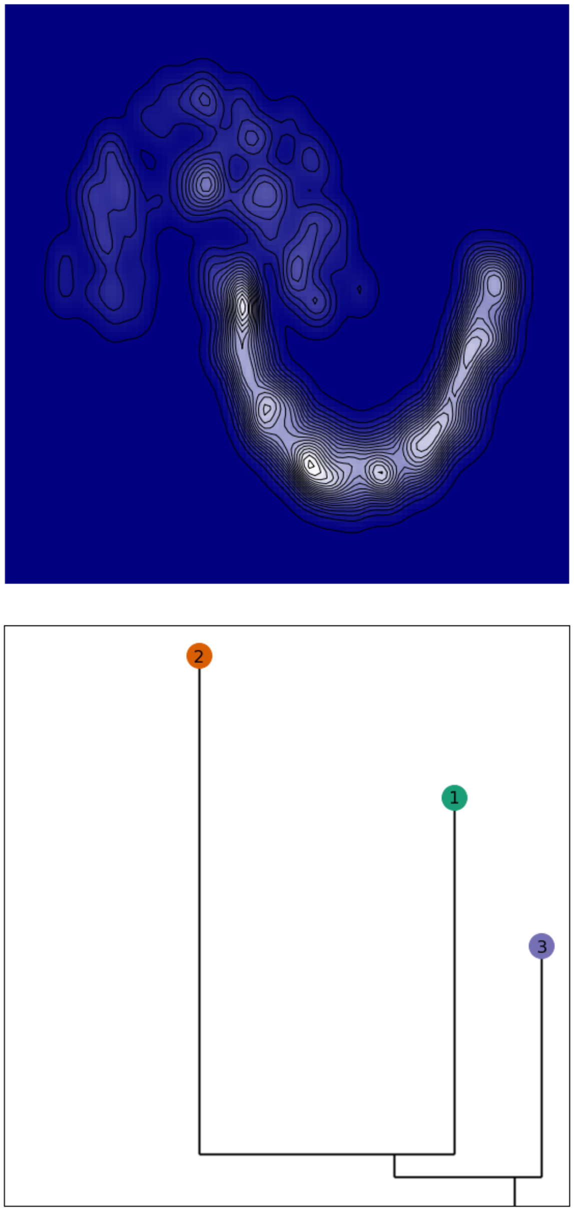


FIG. S4. Analysis of the topography of the Jain [3] data set. A total of 20000 points has been harvested from the probability distribution function shown in the top-left panel, built as a sum of Gaussian functions centered in the original data points. The clusters found with a value of $Z = 2.7$ are shown in top-right panel. The dendrogram and network representations of the topography are in the bottom-left and bottom-right panels respectively.

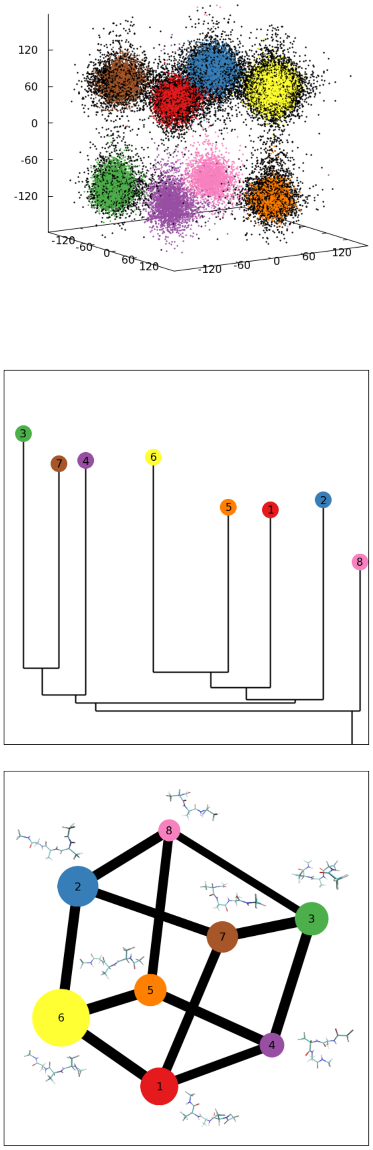


FIG. S5. Analysis of a 2 $\mu$s molecular dynamics trajectory of trialanine in water solution from [4]. The distance between two configurations is estimated from the root mean square difference between the dihedral angles of the backbone, with the differences computed taking into account the periodicity. The estimated intrinsic dimension [5] is 9. In the top panel, the data points are plotted according with the three $\Psi$ dihedral angles and colored according with their clustering assignation. In the middle panel, the dendrogram representation of the topology. In the bottom panel, the network representation with the structures correspondent to the clusters centers represented next to the cluster circles. Please note that the clusters correspond almost perfectly with those found in Ref. [6].

**Text S1. THE CHOICE OF THE PARAMETER Z**

The parameter $Z$, entering in Equation 4 is related with the statistical significance of the clusters found. Its role in real datasets is complex, since the statistical properties of the peaks interplay with the intrinsic dimension, the value of $\hat{k}_i$, the actual shape of the probability density function, etc. With the aim of decoupling some of these effects, we carried out a systematic study on white noise datasets at known dimension, where all the clusters found are, by definition, spurious. Since for such a dataset with $N$ points Pa$k$ will give $\hat{k} = N$ for almost all the points, the test will be carried out with fixed $\hat{k}$, in order to mimic the conditions observed in real data sets. In particular, we study how, for a given $d$ and $\hat{k}$, the choice of $Z$ affects the detection of spurious clusters, since in this case, any density maximum detected by the approach is by construction due to a statistical fluctuation. For $k \to \infty$, the number of density peaks becomes equal to one. If $k$ is finite, the number of peaks grows linearly with the number $N$ of data points. Each (spurious) density peak is characterized by a value of the quantity $\tilde{Z} = \frac{F_c - F_{c,c'}}{\epsilon_c + \epsilon_{c,c'}}$. This quantity, in real world data sets, is taken as a measure of the reliability of the peak: the larger its value, the smaller the probability that the peak is generated by a statistical fluctuation. In Fig. S6A we plot the cumulative probability distribution of $\tilde{Z}$ for different values of $k$ and $d$. These curves imply that if, for example, one fixes a threshold of $Z = 1.5$, one would discard $\sim 96$ % of the spurious peaks for $k = 10$ and $d = 2$ while $\sim 79$ % for $k = 50$ and $d = 8$. In Fig. S6B, we plot which values of $Z$ should be set if one accepts to have on average one spurious cluster every 1000 points. at different values of $k$ and $d$. These curves approximately collapse to a single one, suggesting that the main variable that one should take into account when choosing $Z$ is $d$.

These analysis, strictly speaking, allow understanding the role of $Z$ only if the density is constant. In the general (and relevant) case in which the density varies, they can be considered a qualitative guideline for choosing a value of $Z$.

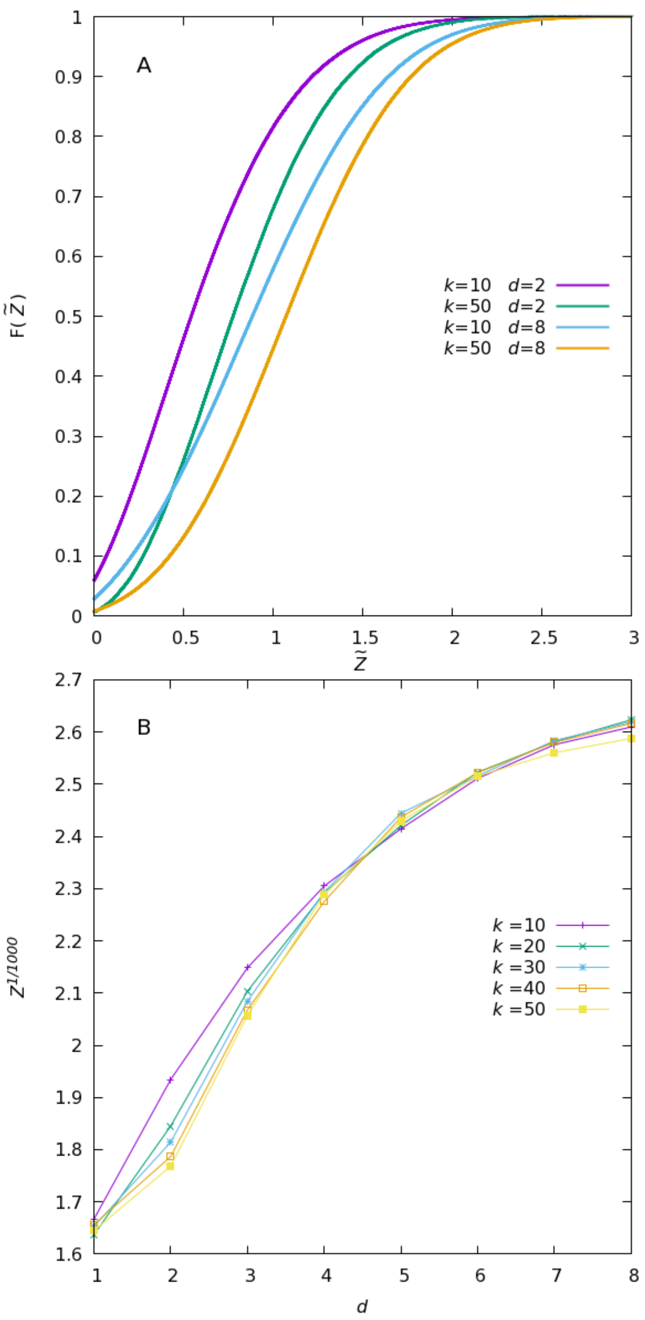


FIG. S6. Effect of parameter $Z$ on the probability of having spurious clusters at constant density. (A) Cumulative probability distributions of $\tilde{Z}$ (see text for definition) as a function of $k$ and $d$. (B) $Z$ values needed for having one spurious cluster each 1000 points in the data set for different values of $k$ and $d$. Note that the cumulates do not start at the point $\tilde{Z} = 0.$. This is an artifacts in the peak detection detection protocol (means that the density of the barrier is higher than the one of the peak), mainly induced by the fact that $k$ has been artificially set to a fixed value.

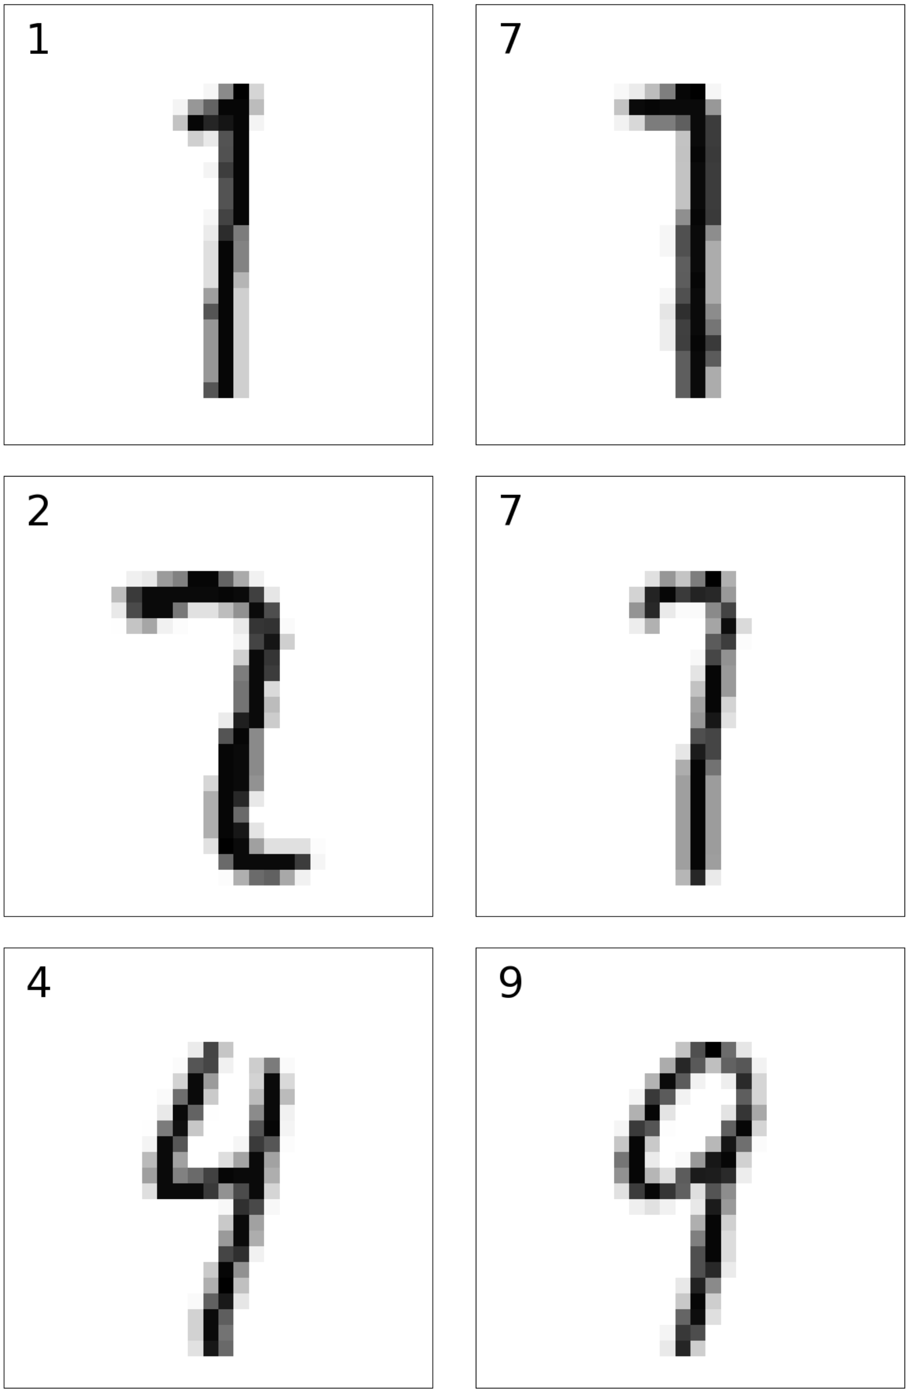


FIG. S7. Some of the handwritten digits with different ground truth but put together in the same cluster by the algorithm.

| | **0** | **1** | **2** | **3** | **4** | **5** | **6** | **7** | **8** | **9** |
|---|---|---|---|---|---|---|---|---|---|---|
| **0** | **996** | 0 | 3 | 3 | 0 | 1 | 17 | 5 | 1 | 3 |
| **1** | 1 | **790** | 39 | 11 | 5 | 4 | 5 | 84 | 16 | 6 |
| **2** | 0 | 5 | **831** | 5 | 0 | 1 | 0 | 2 | 5 | 0 |
| **3** | 2 | 75 | 8 | **967** | 6 | 23 | 1 | 3 | 96 | 64 |
| **4** | 0 | 0 | 0 | 0 | **373** | 0 | 0 | 3 | 2 | 8 |
| **5** | 0 | 1 | 1 | 26 | 0 | **796** | 5 | 0 | 20 | 2 |
| **6** | 1 | 0 | 2 | 2 | 10 | 11 | **986** | 0 | 9 | 0 |
| **7** | 0 | 255 | 101 | 9 | 9 | 6 | 0 | **924** | 11 | 9 |
| **8** | 0 | 0 | 1 | 4 | 0 | 1 | 0 | 0 | **765** | 0 |
| **9** | 1 | 1 | 5 | 5 | 577 | 20 | 0 | 48 | 19 | **886** |

TABLE S1. Confusion matrix between ground truth and cluster classification labeled according with a majority rule for the undersampled (10000 data points) MNIST data set.


[1] A. Gionis, H. Mannila, and P. Tsaparas, ACM Transactions on Knowledge Discovery from Data (TKDD) **1**, 4 (2007).

[2] H. Chang and D.-Y. Yeung, Pattern Recognition **41**, 191 (2008).

[3] A. K. Jain and M. H. Law, in *International conference on pattern recognition and machine intelligence* (Springer, 2005) pp. 1–10.

[4] F. Marinelli, F. Pietrucci, A. Laio, and S. Piana, PLOS Computational Biology **5**, 1 (2009).

[5] E. Facco, M. d'Errico, A. Rodriguez, and A. Laio, Scientific reports **7**, 12140 (2017).

[6] A. Rodriguez and A. Laio, Science **344**, 1492 (2014), http://science.sciencemag.org/content/344/6191/1492.full.pdf.
